# Supplementary material for: Efficient Optical Quantification of Heterogeneous Emitter Ensembles
Source: arXiv:1909.12726 ancillary file (2019-09-27)

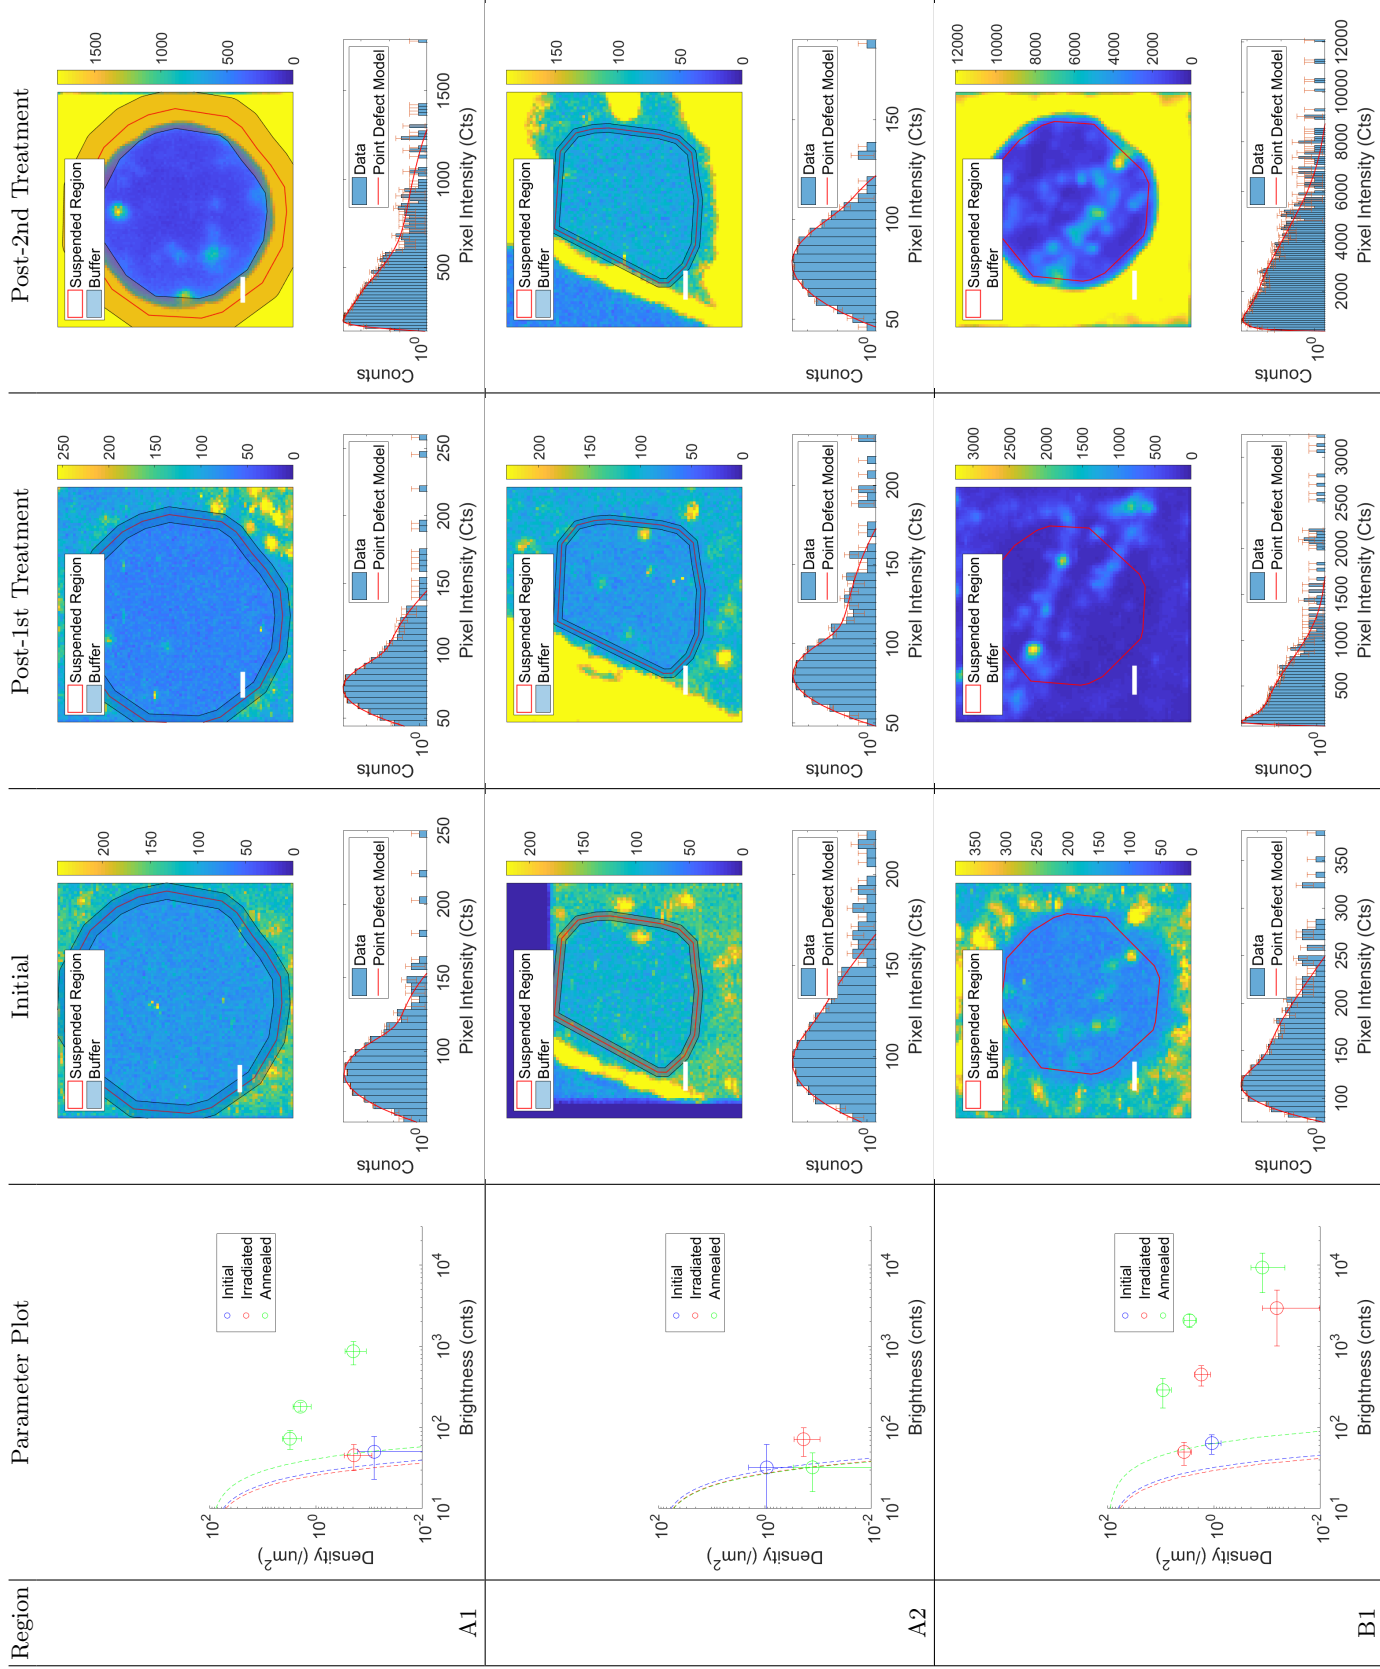

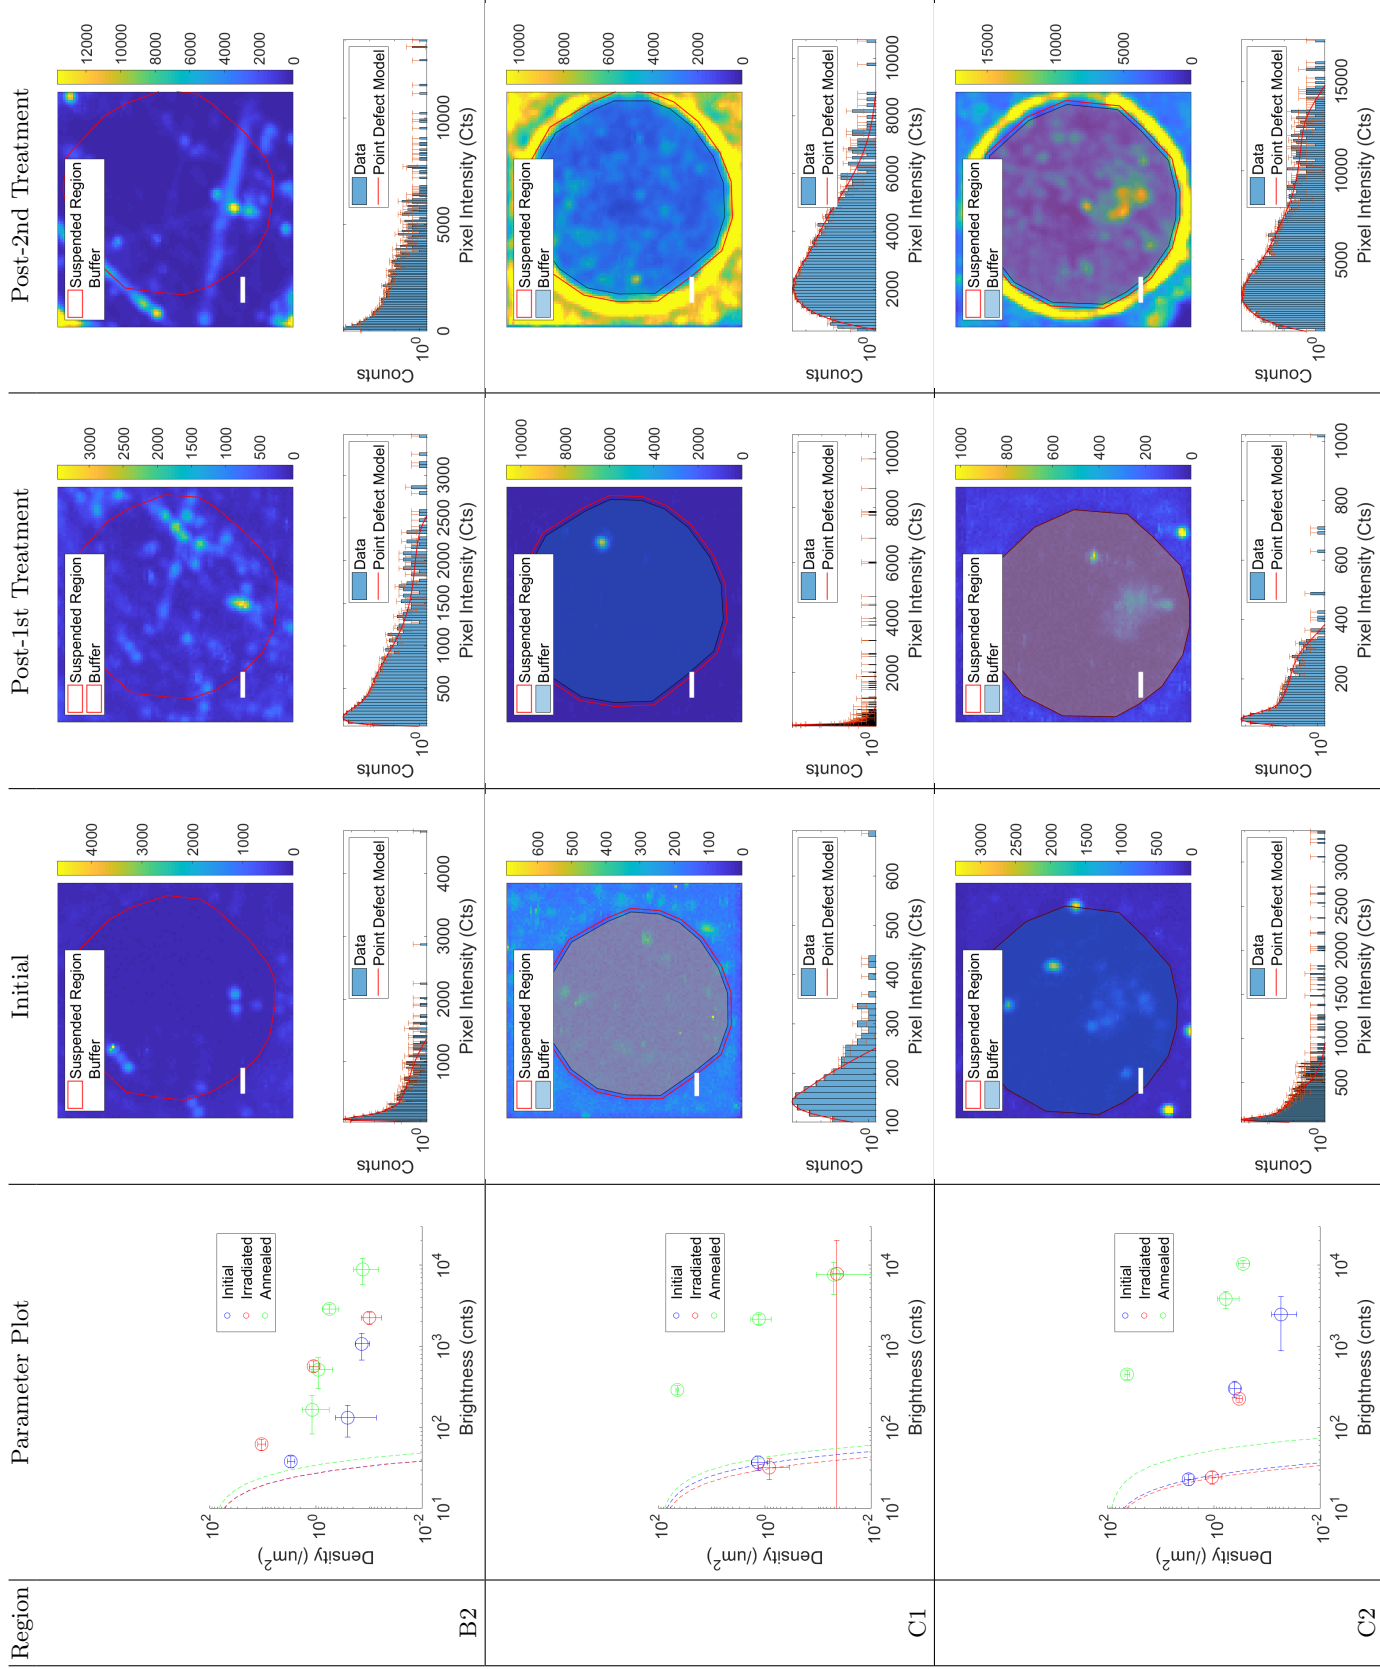

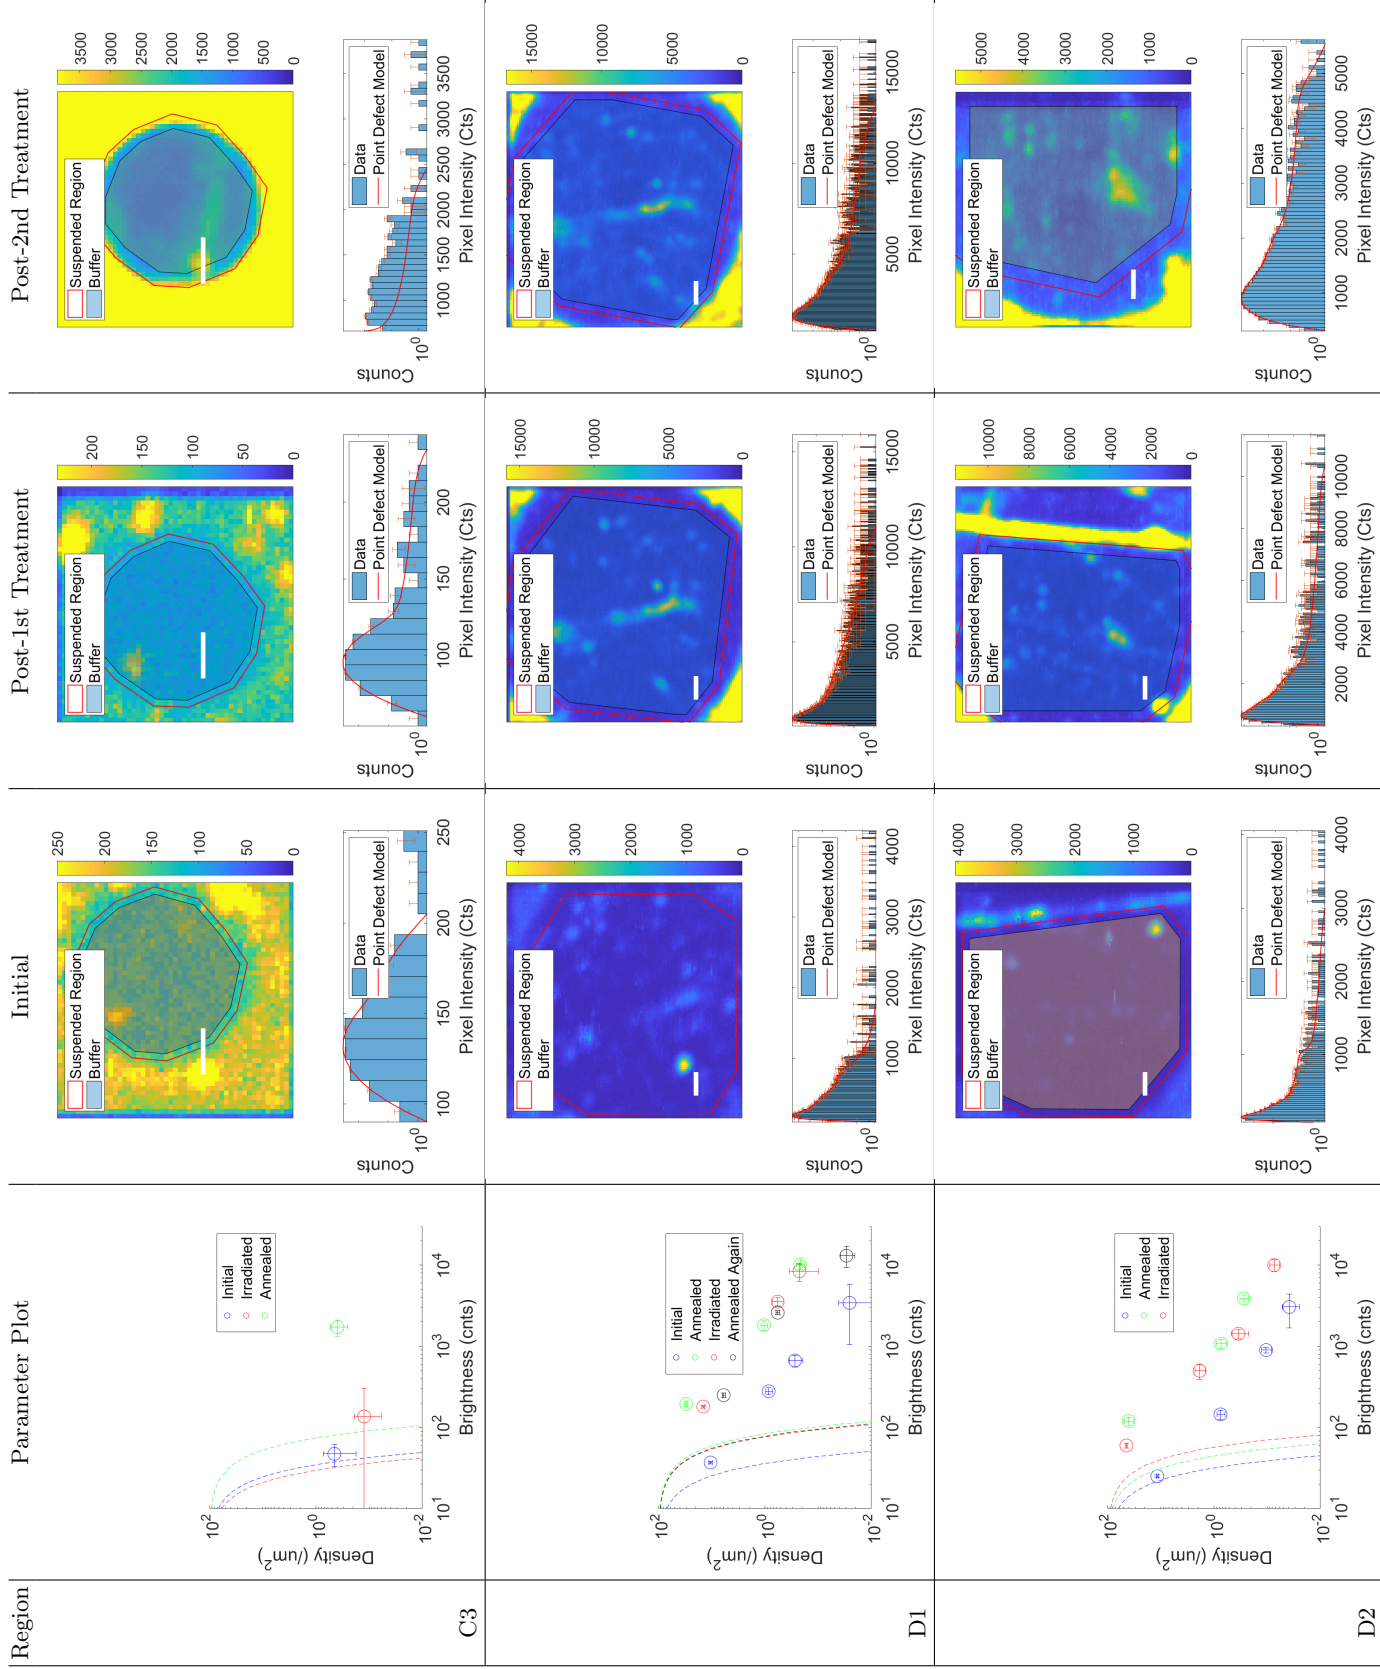

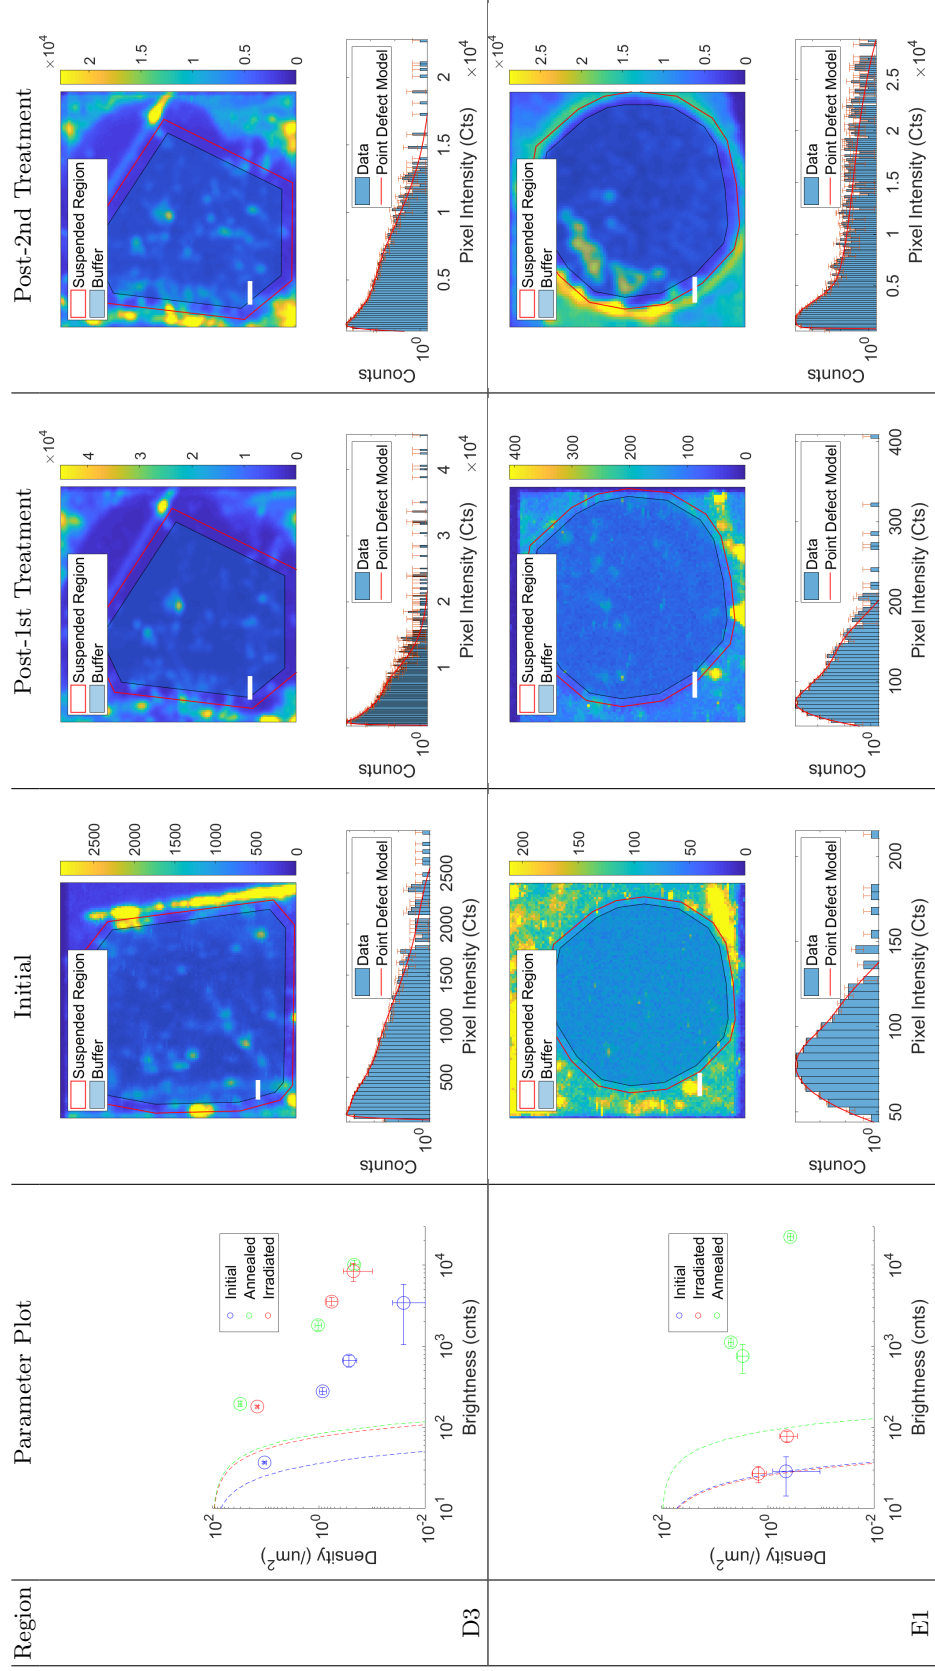

Supplement: Supplementary file 2 [file data.pdf]
